# Supplementary material for: Multireference equation-of-motion driven similarity renormalization group for X-ray photoelectron spectra
Source: arXiv:2509.21646 source file (2025-09-25)
Supplement: Supplementary file 1 [file si.pdf]

**Supporting Information: Multireference equation-of-motion driven similarity renormalization group for X-ray photoelectron spectra**

Shuhang Li,<sup>1</sup> Zijun Zhao,<sup>1</sup> and Francesco A. Evangelista<sup>1, a)</sup>

*Department of Chemistry and Cherry Emerson Center for Scientific Computation,  
Emory University, Atlanta, Georgia 30322, United States*

---

<sup>a)</sup>Electronic mail: francesco.evangelista@emory.edu

## I. CHOICE OF ACTIVE SPACE AND REFERENCE ENERGIES

TABLE S1. The active space and corresponding CASSCF energy (in  $E_h$ ) used in the EOM-DSRG calculations for each molecule. The active space is specified by the number of core and active orbitals per irrep, listed in ‘Cotton ordering’.

| Molecule                      | Core              | Active            | Energy ( $E_h$ ) |
|-------------------------------|-------------------|-------------------|------------------|
| C <sub>2</sub> H <sub>4</sub> | [1,0,0,0,0,0,1]   | [3,2,1,0,0,1,2,3] | -78.237527       |
| CH <sub>4</sub>               | [1,0,0,0]         | [4,0,2,2]         | -40.310940       |
| C <sub>2</sub> H <sub>2</sub> | [1,0,0,0,0,1,0,0] | [3,0,1,1,0,3,1,1] | -77.027293       |
| CH <sub>3</sub> NC            | [6,1]             | [6,2]             | -132.137112      |
| CH <sub>3</sub> OH            | [4,0]             | [8,4]             | -115.305028      |
| CH <sub>3</sub> CN            | [6,1]             | [6,2]             | -132.178361      |
| HCN                           | [2,0,0,0]         | [5,0,2,2]         | -93.102072       |
| CH <sub>2</sub> O             | [2,0,0,0]         | [5,0,2,3]         | -114.112345      |
| CO                            | [2,0,0,0]         | [6,0,2,2]         | -113.018224      |
| CO <sub>2</sub>               | [2,0,0,0,0,1,0,0] | [3,0,1,1,0,3,2,2] | -188.003281      |
| NH <sub>3</sub>               | [2,0]             | [4,2]             | -56.319839       |
| N <sub>2</sub> O              | [4,0,0,0]         | [6,0,4,4]         | -184.141570      |
| H <sub>2</sub> O              | [1,0,0,0]         | [4,0,1,3]         | -76.197095       |
| HF                            | [1,0,0,0]         | [4,0,2,2]         | -100.281376      |
| F <sub>2</sub>                | [1,0,0,0,0,1,0,0] | [2,0,2,2,0,2,2,2] | -199.120916      |

## II. CORE-IONIZATION ENERGIES AND SPECTROSCOPIC FACTORS OF OZONE

Core: [4, 0, 0, 2]; Active: [3, 1, 2, 3]

TABLE S2. Oxygen K-edge core ionization energies ( $\omega$ , eV) and spectroscopic factors ( $S$ ) of ozone calculated using different EOM-DSRG methods. O<sub>C</sub> and O<sub>T</sub> stand for the central and terminal oxygen atoms, respectively.

| Ionization                     | EOM-DSRG-PT2 |       | EOM-DSRG-PT3 |       | EOM-DSRG(2) |       |
|--------------------------------|--------------|-------|--------------|-------|-------------|-------|
|                                | $\omega$     | $S$   | $\omega$     | $S$   | $\omega$    | $S$   |
| O <sub>T</sub> ( $1a_1^{-1}$ ) | 545.49       | 1.476 | 544.64       | 1.431 | 544.62      | 1.435 |
| O <sub>T</sub> ( $1b_2^{-1}$ ) | 545.49       | 1.476 | 544.64       | 1.431 | 544.62      | 1.435 |
| O <sub>C</sub> ( $2a_1^{-1}$ ) | 549.17       | 1.488 | 548.78       | 1.473 | 548.63      | 1.472 |
